# Supplementary material for: Program Synthesis using Natural Language
Source: arXiv:1509.00413 source file (2015-09-01)
Supplement: Supplementary file 1 [file appendix.tex]

\ignore {
\section{Domain Grammars and Example English Inputs}

\newcounter{rowno}
\setcounter{rowno}{0}
\begin{table*}[t!] \small
\begin{center}  
\begin{tabular}{|@{}l@{}l@{}|}
\hline
\multicolumn{1}{|c|}{\small{Grammar}} & \multicolumn{1}{c|}{\small{Benchmarks}} \\
\hline

$
\begin{array}{@{}r@{}c@{}l@{}}
\text{Command} &::= & \text{Insert} \mid \text{Remove} \mid \text{Replace}\\
\text{Insert} &::= & \t{INSERT}(\text{PString}, \text{Position}, \text{IterScope})\\
\text{Remove} &::= & \t{REMOVE}(\text{Selection}, \text{IterScope})\\
\text{Replace} &::= & \t{REPLACE}(\text{Selection}, \text{NewString}, \text{IterScope})\\

\text{PString} &::= & \t{<str>} \mid \t{REPEAT}(\t{<str>}, \t{<num>}) \mid \t{CONCAT}(\t{<str>}, \t{<str>})\\

\text{Position} &::= & (\text{PCond}, \text{Occur}) \mid \t{START} \mid \t{END} \mid \epsilon : \{ \t{START}, \t{END} \}\\
\text{PCond} &::= & \t{BEFORE}(\text{Token}) \mid \t{AFTER}(\text{Token}) \mid  \\
&& \t{BETWEEN}(\text{Token}, \text{SecondToken}) \ldots \\

\text{Token} &::= & \t{<str>} \mid \t{LINE} \mid \t{WORD} \mid \t{NUMBER} \mid \t{WHITESPACE} \ldots\\

\text{SecondToken} &::= & \t{TO}(\text{Token})\\

\text{Occur} &::= & \t{<num>} \mid \text{IntegerSet} \mid \t{FIRST} \mid \t{LAST} \mid \t{ALL}\mid \epsilon : \{ \t{ALL} \} \ldots\\

\text{IntegerSet} & ::= & \t{\{<num>\}}\\

\text{IterScope} &::= & (\text{Scope}, \text{BoolC}, \text{Occur})\\

\text{Scope} &::= & \t{LINES} \mid \t{WORDS}\\

\text{BoolC} &::= & \t{AND}(\text{AtomC}, \text{AtomC}) \mid \t{OR}(\text{AtomC}, \text{AtomC}) \mid \\
&& \t{NOT}(\text{AtomC}) \mid \text{AtomC} \mid \t{TRUE} \mid \epsilon : \{ \t{TRUE} \}\\

\text{AtomC} &::= & \t{STARTS}(\text{Token}) \mid \t{ENDS}(\text{Token}) \mid \t{CONTAINS}(\text{Token}) \mid\\
&& \t{MATCHES}(\text{Token}) \mid \t{BETWEEN}(\text{Token}, \text{SecondToken}) \ldots\\

\text{Selection} &::= & (\text{Token}, \text{BoolC}, \text{Occur})\\

\text{NewString} &::= & \t{BY}(\text{PString})

\end{array}

$

&

\begin{tabular}{|@{}>{\stepcounter{rowno}\therowno. }c@{}l@{}}
& Insert ``:'' after 1st word \\ 
& Add ``\textdollar'' at the beginning of those lines that do not already start with ``\textdollar'' \\ 
& Prepend the line containing ``P.O. BOX'' with ``*'' \\ 
& Add ``..???'' at the last of every 2nd statement \\ 
& For each line, if it ends with ``St.'', replace ``St.'' by ``Street'' \\ 
& In every line, delete the text after ``//'' \\ 
& Remove 1st ``\&'' from every line \\ 
& Remove all the blank lines. \\ 
& Add the suffix ``\_IDM'' to the word right after ``idiom:'' \\ 
& Add an ``!'' followed by a ``?'' at the end of every word \\ 
& Delete all but the 1st occurrence of ``Cook'' \\ 
& Delete the word ``the'' wherever it comes after ``all'' \\ 
& Delete the last 10 lines of a file \\ 
& Remove all symbols which are not numbers \\ 
& Substitute the 4th occurrence of ``foo'' with ``bar'' on each line \\ 
& Replace ``\&'' with ``\&\&'' unless it is inside ``[`` and ``]'' \\ 
& Print all words containing the ``a'' anywhere in the word \\ 
& Extract the word following ``from'' \\ 
& Print data between ``$<$url$>$'' and ``$<$/url$>$'' \\ 
& Print numbers that are immediately followed by the word ``minutes'' \\
\end{tabular}
\\

\hline
\end{tabular}    
\end{center}
\caption{Grammar and Sample Benchmarks for Text Editing domain}
\label{tab:textediting}
\end{table*}

\setcounter{rowno}{0}
\begin{table*}[t!] \small
\begin{center}
    \begin{tabular}{|@{}l@{}|l@{}|}
    \hline
\multicolumn{1}{|c|}{\small{Grammar}} & \multicolumn{1}{c|}{\small{Benchmarks}} \\
\hline

$

\ignore{
\small{
\begin{array}{@{}r@{}c@{}l@{}}

\text{BoolC} &::= & \t{ISODD}(\text{Integer}) \mid \t{ISODDP} \mid \t{ISEVEN}(\text{Integer}) \mid \t{ISEVENP} \mid \\
&& \t{CONTAINS}(\text{CSring}) \mid \t{MATCHFORMAT}(\text{Expr}) \mid \\
&& \t{STARTSWITH}(\text{String}) \mid \t{ENDSWITH}(\text{String}) \mid \\
&& \t{NOT}(\text{BoolC}) \mid \t{AND}(\text{BoolC}, \text{BoolC}) \mid \t{OR}(\text{BoolC}, \text{BoolC}) \mid \\
&& \t{IFTHEN}(\text{BoolC}, \text{BoolC}) \mid \t{IFF}(\text{BoolC}, \text{BoolC}) \mid \\
&& \t{FORALLINT}(\text{BoolC}, \text{BoolC}) \mid \t{EXISTSINT}(\text{BoolC}, \text{BoolC}) \mid \\
&& \t{CONDITIONALPALIN}(\text{BoolC}) \ldots \\

\text{Integer} &::= & \t{<int>} \mid \t{COUNT}(\text{String}) \mid \t{LEN}(\text{String}) \mid \t{LENP} \mid \\
&& \t{DECIMALOFSTRING} \mid \t{BINARYOFSTRING} \ldots \\

\text{String} &::= & \t{<str>} \mid \t{SYMBOLAT}(\text{Integer}) \mid \t{SYMBOLATP} \mid \\
&& \text{ComplexStr} \mid \text{TerminalS} \\

\text{CSring} &::= & \text{String} \mid \text{MultiStr} \\

\text{MultiStr} &::= & \t{ANDSTRINGS}(\text{String}, \text{String}) \mid \t{ORSTRINGS}(\text{String}, \text{String}) \\

\text{ComplexStr} &::=&  \t{CONCAT}(\text{String}, \text{String}) \mid \t{REPEAT}(\text{String}, \text{Times}, \text{RMode}) \\

\text{Times} &::= & \text{Integer} \mid \t{TWICE} \mid \epsilon : \{ \t{TWICE} \}\\

\text{RMode} &::= & \t{RGEQ} \mid \t{RLEQ} \mid \t{REQ} \mid \epsilon : \{ \t{REQ} \}\\

\text{TerminalS} &::= & \t{LASTSYMBOL} \mid \t{FIRSTSYMBOL} \\

\text{Expr} &::= & \t{EXPRESSION} \mid \text{ComplexStr}

\end{array}
}
$

&
}

\begin{tabular}{@{}>{\stepcounter{rowno}\therowno. }c@{}p{6.2cm}}
& The set of strings w such that the symbol at every odd position in w is ``a''\\
& Consider the language L consisting of words that contain ``010''\\
& A string w belongs to the language L precisely when w contains at least 1 ``a'' symbol and does not contain any ``b'' symbols.\\
& The set of strings whose 5th last symbol is ``b''.\\
& w has the same number of occurrences of ``10'' and ``01''\\
& Consider the set of all binary strings where the difference between the number of ``0'' and the number of ``1'' is even.\\
& x begins and ends with the sequence ``aab''.\\
& the set of strings that begin and end with the same symbol\\ 
& w has length at least 3 and its 3rd symbol is ``0''\\ 
& set of x such that any ``a'' in x is followed by a ``b''\\
\end{tabular}
\\

\hline
    \end{tabular}
\end{center}    
\caption{Grammar and Sample Benchmarks for Automata Theory domain}
\label{tab:automata}
\end{table*}

\setcounter{rowno}{0}

\begin{table*}[t!] \small
\begin{center}
    \begin{tabular}{|@{}l@{}|l@{}|}
    \hline
\multicolumn{1}{|c|}{\small{Grammar}} & \multicolumn{1}{c|}{\small{Benchmarks}} \\
\hline

$
\small{
\begin{array}{@{}r@{}c@{}l@{}}

\text{Query} &::= & \text{RowSet} \mid \text{ColSet} \\

\text{RowSet} &::= & \text{AtomRowSet} \mid \t{ROW\_MIN}(\text{Col}, \text{AtomRowSet}) \mid \\
&& \t{ROW\_MAX}(\text{Col}, \text{AtomRowSet}) \mid \\
&& \t{ROW\_MIN\_T}(\text{TCol}, \text{AtomRowSet}) \mid \\
&& \t{ROW\_MAX\_T}(\text{TCol}, \text{AtomRowSet}) \ldots \\

\text{ColSet} &::= & \t{PROJECT}(\text{Col}, \text{RowSet}) \mid (\text{Col}, \text{RowSet}) \\

\text{Col} &::= & \text{AtomCol} \mid \text{AtomColSet} \\

\text{AtomCol} &::= & \t{DEP\_TIME} \mid \t{ARR\_TIME} \mid \\
&& \t{FLIGHT\_NUMBER} \mid \t{AIRLINES} \ldots \\

\text{AtomColSet} &::= & \{ \text{AtomCol} \} \\

\text{TCol} &::= & \t{DEP\_TIME} \mid \t{ARR\_TIME} \mid \epsilon : \{ \t{DEP\_TIME} \} \\

\text{AtomRowSet} &::= & \text{AtomRowPredSet} \mid \text{AtomRowPred} \\

\text{AtomRowPredSet} &::= & \{ \text{AtomRowPred} \} \\

\text{AtomRowPred} &::= & \t{EQ\_DEP}(\text{City}, \text{Time}, \text{Weekday}, \text{Daynum}, \text{Month}) \mid \\
&& \t{EQ\_ARR}(\text{City}, \text{Time}, \text{Weekday}, \text{Daynum}, \text{Month}) \mid \\
&& \t{BETWEEN\_CITIES}(\text{Eq\_Dep\_IMP}, \text{Eq\_Arr\_IMP}) \mid \\
&& \text{ROUND\_TRIP} \ldots \\

\text{Time} &::= & \text{Unit\_Time} \mid \text{Unit\_Time\_Set} \mid \t{ANY} \mid \epsilon : \{ \t{ANY} \} \\

\text{Unit\_Time\_Set} &::= & \{ \text{Unit\_Time} \} \\

\text{Unit\_Time} &::= & \t{TIME} \mid \t{TIME\_GT}(\text{Unit\_Time}) \mid \\
&& \t{TIME\_LT}(\text{Unit\_Time}) \mid \t{TIME\_AROUND}(\text{Unit\_Time})

\end{array}
}
$

&

\begin{tabular}{@{}>{\stepcounter{rowno}\therowno. }c@{}p{6.7cm}}
& i need information on a flight from san francisco to atlanta that would stop in fort worth \\ 
& what ground transportation is there from the airport in atlanta to downtown \\ 
& what is the earliest flight from washington to atlanta leaving on wednesday september fourth \\ 
& show me the flight from detroit to westchester county with the highest one way fare \\ 
& okay we're going from washington to denver first class ticket i'd like to know the cost of a first class ticket \\ 
& i would like to know if i fly on american flight number 813 from boston to oakland if i will stop enroute at another city \\ 
& i would like to make a round trip between washington and san francisco \\ 
& i would like to know what type of aircraft will be used on the morning of july seventh from atlanta to boston \\ 
& are there any direct flights from atlanta to philadelphia arriving in philadelphia about 12 noon \\ 
& i want to know the time of the latest flight i can take from washington to san francisco where i can get a dinner meal \\

\end{tabular}
\\

\hline
    \end{tabular}
\end{center}
\caption{Grammar and Sample Benchmarks for ATIS domain}
\label{tab:atis}
\end{table*}

}
